# Supplementary material for: Fast and Reliable Missing Data Contingency Analysis with Predicate-Constraints
Source: arXiv:2004.04139 source file (2020-04-08)
Supplement: Supplementary file 1 [file appendix.tex]

\appendix
\input{joins.tex}
\input{additional-exp.tex}
